# Supplementary material for: Edited Media Understanding Frames: Reasoning About the Intent and Implications of Visual Misinformation
Source: arXiv:2012.04726 source file (2025-03-26)
Supplement: Supplementary file 1 [file appendix.tex]

\input{sections/8-appendix.tex}
